# Supplementary material for: ROC and AUC with a Binary Predictor: a Potentially Misleading Metric
Source: arXiv:1903.04881 source file (2020-05-05)
Supplement: Supplementary file 1 [file Supplement.pdf]

# Supplemental Material

Here we derive a more detailed derivation of the proofs, which may helpful to teaching this derivation or giving as an exercise.

## Showing a full proof of the strict inequality

$$\begin{aligned} P(X_i > X_j | Y_i = 1, Y_j = 0) &= \\ &P(X_i > X_j | Y_i = 1, Y_j = 0, X_i = \mathbf{0})P(X_i = \mathbf{0} | Y_i = 1, Y_j = 0) \\ &+ P(X_i > X_j | Y_i = 1, Y_j = 0, X_i = \mathbf{1})P(X_i = \mathbf{1} | Y_i = 1, Y_j = 0) \\ &= P(X_i > X_j | Y_i = 1, Y_j = 0, X_i = 1)P(X_i = 1 | Y_i = 1, Y_j = 0) \end{aligned} \quad (1)$$

as  $P(X_i > X_j | Y_i = 1, Y_j = 0, X_i = 0) = 0$  because  $X_i$  and  $X_j$  are in  $\{0, 1\}$ . We see that  $P(X_i = 1 | Y_i = 1, Y_j = 0)$  in equation (1) is the sensitivity by independence:

$$\begin{aligned} P(X_i = 1 | Y_i = 1, Y_j = 0) &= P(X_i = 1 | Y_i = 1) \\ &= \frac{TP}{TP + FN} \\ &= \text{sensitivity} \end{aligned}$$

and that  $P(X_i > X_j | Y_i = 1, Y_j = 0, X_i = 1)$  in equation (1) is the specificity:

$$\begin{aligned} P(X_i > X_j | Y_i = 1, Y_j = 0, X_i = 1) &= \\ &P(X_i > X_j | Y_i = 1, Y_j = 0, X_i = 1, X_j = \mathbf{1})P(X_j = \mathbf{1} | Y_i = 1, Y_j = 0, X_i = 1) \\ &+ P(X_i > X_j | Y_i = 1, Y_j = 0, X_i = 1, X_j = \mathbf{0})P(X_j = \mathbf{0} | Y_i = 1, Y_j = 0, X_i = 1) \\ &= P(X_i > X_j | Y_i = 1, Y_j = 0, X_i = 1, X_j = 0)P(X_j = 0 | Y_i = 1, Y_j = 0, X_i = 1) \\ &= P(X_j = 0 | Y_i = 1, Y_j = 0, X_i = 1) \\ &= P(X_j = 0 | Y_j = 0) \\ &= \frac{TN}{TN + FP} \\ &= \text{specificity} \end{aligned}$$

as the first probability is zero as  $X_i = X_j = 1$ . We combine these two to show that equation (1) reduces to:

$$P(X_i > X_j | Y_i = 1, Y_j = 0) = \text{specificity} \times \text{sensitivity}$$

Thus, using the definition as  $P(X_i > X_j | Y_i = 1, Y_j = 0)$ , the AUC of a binary predictor is simply the sensitivity times the specificity.

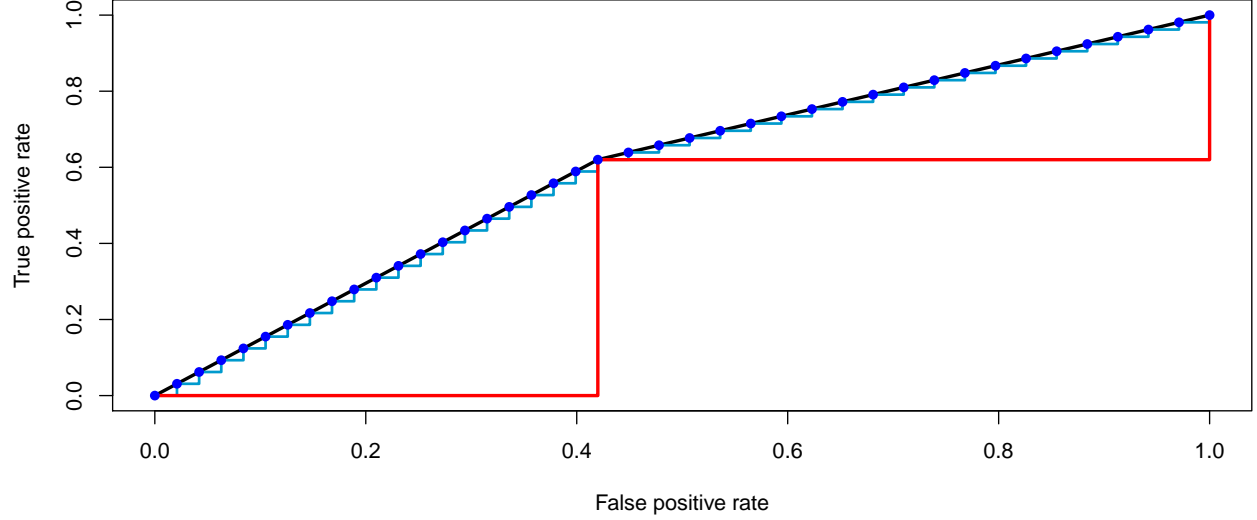

Figure 1: ROC curve of the data in the binary versus extreme categorical variable.

## Showing a the additional ties

$$\begin{aligned}
P(X_i = X_j | Y_i = 1, Y_j = 0) &= P(X_i = X_j | Y_i = 1, Y_j = 0, X_i = \mathbf{1}, X_j = \mathbf{1}) \\
&\quad + P(X_i = X_j | Y_i = 1, Y_j = 0, X_i = \mathbf{0}, X_j = \mathbf{0}) \\
&= P(X_i = \mathbf{1} | Y_i = 1) P(X_j = \mathbf{1} | Y_j = 0) \\
&\quad + P(X_i = \mathbf{0} | Y_i = 1) P(X_j = \mathbf{0} | Y_j = 0) \\
&= (\text{sensitivity} \times (1 - \text{specificity})) \\
&\quad + ((1 - \text{sensitivity}) \times \text{specificity})
\end{aligned}$$

## A more extreme example of differences with categorical variables

We can make a more extreme (yet contrived) example than the categorical example we presented before. Let us say we have 20000 samples in the data set and we have a binary predictor with the a distribution against the outcome as in Table 1.

Table 1: A simple 2x2 table of a binary predictor (rows) versus a binary outcome (columns)

|   | 0    | 1    |
|---|------|------|
| 0 | 5800 | 3800 |
| 1 | 4200 | 6200 |

Let us assume we have a continuous predictor (e.g. age), but only had 20 unique values observed, so we can also consider it empirically discrete. Here we see the frequency table in Table 2.

When we create the ROC curves, they have identical curves when accounting for ties (black). The red and blue lines represents the ROC curves for the pessimistic estimation for the binary (red) and continuous though discrete (blue) variables. We see they give vastly different results. As the continuous predictor can actually achieve sensitivity/specificity combinations on the black line, it may make more sense using the linear interpolation, but the pessimistic approach ROC curve is similar.

Table 2: A simple 2x2 table of a discrete predictor (rows) versus a binary outcome (columns)

|        | 0   | 1   |
|--------|-----|-----|
| 0.0277 | 290 | 190 |
| 0.0483 | 290 | 190 |
| 0.0586 | 290 | 190 |
| 0.0691 | 290 | 190 |
| 0.08   | 290 | 190 |
| 0.0827 | 290 | 190 |
| 0.0931 | 290 | 190 |
| 0.0964 | 290 | 190 |
| 0.1463 | 290 | 190 |
| 0.1476 | 290 | 190 |
| 0.1534 | 290 | 190 |
| 0.1747 | 290 | 190 |
| 0.2109 | 290 | 190 |
| 0.2145 | 290 | 190 |
| 0.2387 | 290 | 190 |
| 0.2448 | 290 | 190 |
| 0.2493 | 290 | 190 |
| 0.2619 | 290 | 190 |
| 0.2795 | 290 | 190 |
| 0.2894 | 290 | 190 |
| 0.2911 | 210 | 310 |
| 0.3169 | 210 | 310 |
| 0.3191 | 210 | 310 |
| 0.3517 | 210 | 310 |
| 0.3597 | 210 | 310 |
| 0.3761 | 210 | 310 |
| 0.3813 | 210 | 310 |
| 0.4552 | 210 | 310 |
| 0.5264 | 210 | 310 |
| 0.6066 | 210 | 310 |
| 0.6136 | 210 | 310 |
| 0.6393 | 210 | 310 |
| 0.6572 | 210 | 310 |
| 0.6971 | 210 | 310 |
| 0.7799 | 210 | 310 |
| 0.7936 | 210 | 310 |
| 0.8197 | 210 | 310 |
| 0.8915 | 210 | 310 |
| 0.9026 | 210 | 310 |
| 0.9957 | 210 | 310 |
